# Supplementary material for: Exact Simulation of Longitudinal Data from Marginal Structural Models
Source: arXiv:2502.07991 source file (2025-04-24)
Supplement: Supplementary file 1 [file appendices.tex]

\subsection{Simulate \protect\((L_2,A_2,Y_3 \cmid Z,\bar{L}_1,\bar{A}_1, Y_2 = 0)\protect\)}

We simulate $(L_2,A_2)$ given $\cmid Z,\bar{L}_1,\bar{A}_1, Y_2 = 0)$ similarly to the previous time step k=1, here we put more focus on simulating $Y_3$ and the copula $ c^*_{Y_3 \bar{L}_2\mid \bar{A}_1, Z}(u^*_{Y_1},u_{L_0},u_{L_1}; \bs \theta)$.
\begin{align}
    p(l_2,a_2,y_3 \cmid z, \bar{l}_1, \bar{a}_1)  &=  p_{L_2\mid Z,\bar{L}_1,\bar{A}_1} (l_2 \cmid z,\bar{l}_1, \bar{a}_1) \cdot 
    p_{A_2 \mid Z,\bar{L}_2,\bar{A}_1}(a_2 \cmid z,\bar{l}_2, \bar{a}_1) \label{eqn:k_2_past}\\
    &\cdot p_{Y_3\mid \bar{A}_2,Z}^*(y_3\cmid do(\bar{a}_2),z)\\
    &\cdot c^*_{Y_3 \bar{L}_2\mid \bar{A}_2, Z}(u^*_{Y_3},u_{L_0},u_{L_1},u_{L_2}; \bs \theta) \label{eqn:k_2_cop},
\end{align}
where we use a pair-copula construction as depicted in Figure \ref{fig:pcc_k_2_cop} for the four-dimensional copula in (\ref{eqn:k_2_cop}). Since there many possible D-vine PCCs for this given copula, where we can rearrange the positions of the four variables, we recommend the specific PCC shown in Figure \ref{fig:pcc_k_2_cop}. This choice is advantageous because the inputs into the pair-copula that do not involve $Y_3$, including the quantiles of $F_{L_1\mid L_0}$ and $F_{L_2\mid L_0,L1}$, are readily available and correspond directly to the uniform random variables $w$'s used to sequentially generate the $L_k$'s. Compared to other orderings of the variables,  this particular D-vine PCC offers the convenience of using the pre-generated uniform variables without the need to compute additional input quantiles for the copulas.

\begin{figure}
    \centering
    \begin{tikzpicture}
    
  % First row
    \node[circle, draw, minimum size = 1cm, ] (1) {$L_2$};
    \node[circle, draw, minimum size = 1cm, right=2cm of 1] (2) {$L_1$};
    \node[circle, draw, minimum size = 1cm, , right=2cm of 2] (3) {$L_0$};
    \node[circle, draw, minimum size = 1cm, , right=2cm of 3] (4) {$Y_3$};
    \node[  minimum size = 1cm , right=2cm of 4] (T1) {$T_1$};

    \draw (1) -- node[above] {$L_1 L_2$} (2);
    \draw (2) -- node[above] {$L_0 L_1$} (3);
    \draw (3) -- node[above] {$L_0 Y_3$} (4);

  % Second row
    \node[circle, draw, minimum size = 1cm, below right =1cm and 1cm of 1] (12) {$L_1 L_2$};
    \node[circle, draw, minimum size = 1cm, below right =1cm and 1cm of 2] (23) {$L_0 L_1$};
        \node[circle, draw, minimum size = 1cm, below right =1cm and 1cm of 3] (34) {$L_0 Y_3$};
    \node[  minimum size = 1cm , below=1cm of T1] (T2) {$T_2$};
    \draw (12) -- node[above] {$L_0L_2\mid L_1$} (23);
    \draw (23) -- node[above] {$L_1Y_3\mid L_0$} (34);
  
  % Third row
  \node[circle, draw, minimum size = 0.8cm, below right =1cm and 1cm of 12] (13_2) {\tiny $L_0 L_2 \mid L_1$};
  \node[circle,draw, minimum size = 1cm, below right =1cm and 1cm of 23]  (24_3) {\tiny $L_1 Y_3 \mid L_0$};
    \node[  minimum size = 1cm , below=1cm of T2] (T3) {$T_3$};
  \draw (13_2) -- node[above] {\small $L_2 Y_3 \mid \bar{L}_1$} (24_3);
  
\end{tikzpicture}
    \caption{A D-vine PCC of $c^*_{Y_3 \bar{L}_2\mid \bar{A}_2, Z}$ in (\ref{eqn:k_2_cop}).  Note that all the copulas in this figure are conditioned on $do(\bar{A}_2)$, $Z$ and $Y_2 =0$ but these conditioning variables are omitted for brevity.}
    \label{fig:pcc_k_2_cop}
\end{figure}

The steps to simulate from this factorization are as follows:
\begin{enumerate}[label=(\roman*)]
    \item Generate three uniform random numbers $w_7,w_8,w_{9}$.
    \item Simulate $(l_2,a_2)$ sequentially according to (\ref{eqn:k_2_past}):
        \begin{enumerate}
            \item $l_2 = F^{-1}_{L_2\mid Z,\bar{L}_1,\bar{A}_1} (w_7 \cmid z,\bar {l}_1,\bar {a}_1) $
            \item $a_2 = F^{-1}_{A_2 \mid Z,\bar{L}_2,\bar{A}_1}(w_8 \cmid z,\bar {l}_2,\bar {a}_1)$
        \end{enumerate}
    \item Simulate the marginal quantile of $Y_2$ from the copula in (\ref{eqn:k_2_cop}) following the PCC shown in Figure \ref{fig:pcc_k_2_cop}: 
    \begin{enumerate}
        \item Starting from Tree 3, first simulate $C_{Y_3\mid L_0L_1}$ from the copula $c^*_{L_2 Y_3 \mid L_0L1}$
            \begin{align}
                 C_{Y_3\mid \bar{L}_1}(u^*_{Y_3} \cmid u_{L_0},u_{L_1}) &= h^{-1}(w_{9}, F_{L_2\mid \bar{L}_1}(l_2\cmid \bar{l}_1)); \bs \theta_{31})\\
                 & = h^{-1}(w_{9}, w_7; \bs \theta_{31}),
            \end{align}
            where $w_7 =F_{L_2\mid \bar{L}_1}(l_2\cmid \bar{l}_1)$ by design as $L_2$ was simulated in step (ii)(a) using this conditional distribution.
        \item Then, in Tree 2, simulate $C_{Y_3\mid L_0}$ from the copula 
        $c^*_{L_1 Y_3 \mid L_0}$:
            \begin{align}
                 C_{Y_3\mid L_0}(u^*_{Y_3} \cmid u_{L_0}) &= h^{-1}( C_{Y_3\mid \bar{L}_1}, F_{L_1\mid L_0}(l_1\cmid l_0)); \bs \theta_{22})\\
                 & = h^{-1}(C_{Y_3\mid \bar{L}_1}, w_4; \bs \theta_{22}),
            \end{align}
        \item in Tree 1, simulate the marginal quantile $u^*_{Y_3}$ from the copula $c^*_{L_0 Y_3}$:
            \begin{align}
             u^*_{Y_3} &= h^{-1}( C_{Y_3\mid L_0}, F_{L_0}(l_0); \theta_{12})\\
             &= h^{-1}( C_{Y_3\mid L_0}, w_1; \theta_{13})
        \end{align}
    \end{enumerate}

    \item Invert the MSM CDF to obtain $y_3$:
        \begin{align*}
            y_3 =  F_{Y_3\mid \bar{A}_2, Z}^{*-1}(u^*_{Y_3}\cmid do(\bar{a}_2),z).
        \end{align*}
\end{enumerate}

\begin{landscape} % Start landscape mode

\begin{figure}
    \centering
    \begin{tikzpicture}
    
  % First row
    \node[circle, draw, minimum size = 1.5cm, ] (1) {$L_k$};
    \node[circle, draw, minimum size = 1.5cm, right=2cm of 1] (2) {$L_{k-1}$};
    \node[circle, draw, minimum size = 1.5cm, , right=2cm of 2] (3) {$L_{k-2}$};
    % \node[circle, draw, minimum size = 1cm, , right=2cm of 3] (4) {$L_{k-3}$};
    \node[circle, minimum size = 1.5cm, , right=0.5cm of 3] (dots1) {$\cdots$};
        \node[circle, draw, minimum size = 1.5cm, , right=0.5cm of dots1] (4) {$L_2$};
    \node[circle, draw, minimum size = 1.5cm, , right=2cm of 4] (5) {$L_1$};
    \node[circle, draw, minimum size = 1.5cm, , right=2cm of 5] (6) {$L_0$};
    \node[circle, draw, minimum size = 1.5cm, , right=2cm of 6] (7) {$Y_{k+1}$};
    \node[  minimum size = 1cm , right=2cm of 7] (T1) {$T_1$};

    \draw (1) -- node[above] {$L_k L_{k-1}$} (2);
    \draw (2) -- node[above] {$L_{k-1} L_{k-2}$} (3);
    \draw (3) -- node[above] {} (dots1);
     % \draw (4) -- node[above] {} (dots1);
      \draw (dots1) -- node[above] {} (4);
       \draw (4) -- node[above] {$L_2L_1$} (5);
    \draw (5) -- node[above] {$L_1 L_0$} (6);
    \draw (6) -- node[above] {$L_0 Y_{k+1}$} (7);

  % Second row
    \node[circle, draw, minimum size = 1.5cm, below right =1cm and 1cm of 1,label= below:$L_k L_{k-1}$] (21) {$\Theta_{2,1}$};
    \node[circle, draw, minimum size = 1.5cm, below right =1cm and 1cm of 2,label= below:$L_{k-1} L_{k-2}$] (22) {$\Theta_{2,2}$};
    \node[circle, minimum size = 1.5cm, , below right =1cm and -0.5cm of dots1] (dots2) {$\cdots$};
    \node[circle, draw, minimum size = 1.5cm, below right =1cm and 1cm of 4,label= below:$L_1L_2$] (23) {$\Theta_{2,{k-1}}$};

    \node[circle, draw, minimum size = 1.5cm, below right =1cm and 1cm of 5,label= below:$L_1 L_0$] (24) {$\Theta_{2,k}$};
    \node[circle, draw, minimum size = 1.5cm, below right =1cm and 1cm of 6,label= below:$L_0 Y_{k+1}$] (25) {$\Theta_{2,k+1}$};
    
    \node[  minimum size = 1cm , below=1.3cm of T1] (T2) {$T_2$};
    \draw (21) -- node[above] {$L_kL_{k-2}\mid L_{k-1}$} (22);
    \draw (22) -- node[above] {} (dots2);
    \draw (dots2) -- node[above] {} (23);
    \draw (23) -- node[above] {$L_2L_0\mid L_1$} (24);
    \draw (24) -- node[above] {$L_1Y_{k+1}\mid L_0$} (25);
  
  % Third row

    \node[circle, draw, minimum size = 1.5cm, below right =1cm and 1cm of 21,label= below:$L_k L_{k-2} \mid L_{k-1}$] (31) {$\Theta_{3,1}$};
    \node[circle, minimum size = 1.5cm, , below right =1cm and -0.5cm of dots2] (dots3) {$\cdots$};
    \node[circle, draw, minimum size = 1.5cm, below right =1cm and 1cm of 23,label= below:$L_2L_0 \mid L_1$] (32) {$\Theta_{3,k-1}$};
    \node[circle, draw, minimum size = 1.5cm, below right =1cm and 1cm of 24,label= below:$L_1Y_{k+1} \mid L_0$] (33) {$\Theta_{3,k}$};
    \node[  minimum size = 1cm , below=1.3cm of T2] (T3) {$T_3$};
  \draw (31) -- node[above] {} (dots3);
    \draw (dots3) -- node[above] {} (32);
    \draw (32) -- node[above] {\small $L_2 Y_{k+1}  \mid \bar{L}_1$} (33);

    % Forth row
    \node[circle, draw, minimum size = 1.5cm, below left =1cm and 1cm of 33,label= below:$L_2 Y_{k+1} \mid \bar{L}_1$] (41) {$\Theta_{4,{k-1}}$};
    \node[  minimum size = 1cm , left=1cm of 41] (40) {};
    \node[  minimum size = 1cm , below=1.3cm of T3] (T4) {$T_4$};

    \draw (40) -- node[above] {} (41);
    
    % Sixth row
    \node[circle, draw, minimum size = 1.5cm, below left =1cm and 1cm of 41,label= below:$L_3 Y_{k+1} \mid \bar{L}_2$] (51) {$\Theta_{5,{k-2}}$};
    \node[  minimum size = 1cm , left=1cm of 51] (50) {};
    \node[  minimum size = 1cm , below=1.3cm of T4] (T5) {$T_5$};

    \node[circle, minimum size = 1.5cm, below left =1cm and 1cm of 51] (61) {$\dots$};
    \draw (50) -- node[above] {} (51);

    % % Fifth row
    % \node[circle, draw, minimum size = 1.5cm, below left =1cm and 1cm of 41,label= below:$L_3 Y_{k+1} \mid \bar{L}_2$] (51) {$\Theta_{5,{k-2}}$};

    % % Sixth row
    % \node[circle, draw, minimum size = 1.5cm, below left =1cm and 1cm of 51,label= below:$L_4 Y_{k+1} \mid \bar{L}_3$] (61) {$\Theta_{6,{k-3}}$};

    % Final row
    % \node[circle, minimum size = 1.5cm, below left =1cm and 1cm of 61] (71) {$\dots$};

    %     % Final row
    \node[circle, draw, minimum size = 1.5cm, below left =1cm and 1cm of 61,label= below:$L_k Y_{k+1} \mid \bar{L}_{k-1}$] (71) {$\Theta_{k+2,1}$};
    \node[  minimum size = 1cm , below=2.5cm of T5] (Tk) {$T_{k+2}$};
        % \node[circle, draw, minimum size = 1.5cm, below left =1cm and 1cm of 51,label= below:$L_k Y_{k+1} \mid \bar{L}_{k-1}$] (71) {$\Theta_{6,{k-3}}$};
    
\end{tikzpicture}
    \caption{A D-vine PCC of $c^*_{Y_3 \bar{L}_2\mid \bar{A}_2, Z}$ in (\ref{eqn:k_2_cop}).  Note that all the copulas in this figure are conditioned on $do(\bar{A}_2)$, $Z$ and $Y_2 =0$ but these conditioning variables are omitted for brevity.}
    \label{fig:pcc_k_2_cop}
\end{figure}

\end{landscape} % End landscape mode
